# Supplementary material for: Uncertainty and Structure in Neural Ordinary Differential Equations
Source: arXiv:2305.13290 source file (2023-05-22)
Supplement: Supplementary file 4 [file supp_bq.tex]

\section{Bayesian Quadrature}
We now provide a short introduction to BQ and the derivation of the kernel mean embedding for truncated Gaussians.
\subsection{Introduction to Bayesian quadrature}
\label{sec:bq_details}

Recall that we are interest in approximating the integral $\Pi[f] = \int_{\mathcal{X}} f(x) \pi(x) dx$. BQ works by placing a $\mathcal{GP}(m, k)$ on $f$, i.e. a GP with mean function $m:\mathcal{X} \rightarrow \mathbb{R}$ and covariance functions (or kernel) $k : \mathcal{X}  \times \mathcal{X} \rightarrow \mathbb{R}$.
Then, given observation $\{x_i,f(x_i)\}_{i=1}^n$, we can compute the posterior mean and variance on the value of $\Pi[f]$ as
\begin{talign*}
	\mathbb{E}\left[ \Pi[f] \right] &= \int_{\mathcal{X}} \left(m(x) + k(x, x_{1:n}) k(x_{1:n},x_{1:n})^{-1} (f(x_{1:n})-m(x_{1:n}))\right) \pi(x) dx\\
	&= \Pi[m] + \Pi[k(\cdot, x_{1:n})] k(x_{1:n},x_{1:n})^{-1} (f(x_{1:n})-m(x_{1:n})),\\
	\mathbb{V}\left[ \Pi[f] \right] &=
	\int_{\mathcal{X}} \int_{\mathcal{X}} \left(k(x, x') - k(x, x_{1:n}) k(x_{1:n},x_{1:n})^{-1}  k(x_{1:n}, x')\right) \pi(x) \pi(x') dx dx'\\
	&= \Pi\bar{\Pi}[k] + \Pi[k(\cdot, x_{1:n})] k(x_{1:n},x_{1:n})^{-1} \Pi[k(x_{1:n}, \cdot)],
\end{talign*}
where $f(x_{1:n}) \in \mathbb{R}^n$ with $[f(x_{1:n})]_{i} = f(x_i)$, $m(x_{1:n}) \in \mathbb{R}^n$ with $[m(x_{1:n})]_{i} = m(x_i)$,  $k(x_{1:n},x)^\top = k(x,x_{1:n})\in \mathbb{R}^n$ with $[k(x,x_{1:n})]_i = k(x,x_{i})$,  $k(x_{1:n}, x_{1:n}) \in \mathbb{R}^{n \times n}$ with $[k(x_{1:n}, x_{1:n})]_{ij} = k(x_i,x_j)$ for all $i,j$ in $\{1,\ldots,n\}$. Finally, $\Pi\bar{\Pi}[k] = \int_{\mathcal{X}} \int_{\mathcal{X}} k(x, x')  \pi(x) \pi(x') dx dx'$. 


Clearly, the expressions above can only be used if $\Pi[k(\cdot, x)]$, called the kernel mean embedding, and $\Pi\bar{\Pi}[k]$, called the initial error, are known in closed-form. This is only possible for some combinations of distribution $\pi$ and covariance function $k$. For example, if $\mathcal{X}=\mathbb{R}^d$, $\pi$ is a Gaussian and $k$ is the RBF-kernel, then the expressions above can be computed analytically. A more challenging case is that of truncated Gaussian distributions. In the next section, we show that the kernel mean embedding can be derived in that case.

\subsection{Kernel Mean Embedding for Truncated Gaussians}
\label{sec:bq_truncated_gaussians}
For truncated Gaussian distributions and the RBF kernel, we can compute the posterior mean but not the posterior variance.
Here we consider the 1-dimensional case with $\mathcal{X} = [a, b]$ which can be extended to the $d$-dimensinal case for isotropic Gaussians. 
We provide the expression for the kernel mean embedding: $\Pi[k(\cdot, x)] = \int_{\mathcal{X}} k(x', x) \pi(x')dx'$. We consider the case when $\pi$ is a truncated Gaussian and introduce the following notation:
\begin{talign*}
	\pi(x) = \frac{\phi(x, \mu, \sigma)}{\Phi(\frac{b-\mu}{\sigma}) - \Phi(\frac{a -\mu}{\sigma})}
\end{talign*}
where $\phi(x) = (\sqrt{2 \pi} \sigma)^{-1} \exp (-(x-\mu)^2/2\sigma^2)$ and  $\Phi(x) = \frac{1}{2}(1 + \text{erf}(x/\sqrt{2}))$. 

We use $Z$ to denote the normalization constant
\begin{talign*}
	Z(a,b,\mu, \sigma) = \Phi\left(\frac{b-\mu}{\sigma}\right) - \Phi\left(\frac{a -\mu}{\sigma}\right)
\end{talign*}
We rewrite the RBF kernel using the above identities $k(x, x') = \exp\left(-(x-x')^2/2l^2\right) = l \sqrt{2 \pi} \phi(x, x', l)$. We can now express the kernel mean embedding as:
\begin{talign*}
	\Pi[k(\cdot, x)] = \int_a^b  l \sqrt{2 \pi} \phi(x, x', l) \frac{\phi(x', \mu, \sigma)}{Z(a, b, \mu, \sigma)} dx' = C l \sqrt{2 \pi}\int_a^b \frac{\phi(x', \tilde{\mu}, \tilde{\sigma})}{Z(a, b, \mu, \sigma)} dx' = l \sqrt{2 \pi} C \frac{Z(a, b, \tilde{\mu}, \tilde{\sigma})}{Z(a, b, \mu, \sigma)},
\end{talign*}
where For truncated Gaussian distributions and the RBF kernel, we can compute the posterior mean but not the posterior variance.
Here we consider the 1-dimensional case with $\mathcal{X} = [a, b]$ which can be extended to the $d$-dimensinal case for isotropic Gaussians. 
We provide the expression for the kernel mean embedding: $\Pi[k(\cdot, x)] = \int_{\mathcal{X}} k(x', x) \pi(x')dx'$. We consider the case when $\pi$ is a truncated Gaussian and introduce the following notation:
\begin{talign*}
	\pi(x) = \frac{\phi(x, \mu, \sigma)}{\Phi(\frac{b-\mu}{\sigma}) - \Phi(\frac{a -\mu}{\sigma})}
\end{talign*}
where $\phi(x) = (\sqrt{2 \pi} \sigma)^{-1} \exp (-(x-\mu)^2/2\sigma^2)$ and  $\Phi(x) = \frac{1}{2}(1 + \text{erf}(x/\sqrt{2}))$. 

We use $Z$ to denote the normalization constant
\begin{talign*}
	Z(a,b,\mu, \sigma) = \Phi\left(\frac{b-\mu}{\sigma}\right) - \Phi\left(\frac{a -\mu}{\sigma}\right)
\end{talign*}
We rewrite the RBF kernel using the above identities $k(x, x') = \exp\left(-(x-x')^2/2l^2\right) = l \sqrt{2 \pi} \phi(x, x', l)$. We can now express the kernel mean embedding as:
\begin{talign*}
	\Pi[k(\cdot, x)] = \int_a^b  l \sqrt{2 \pi} \phi(x, x', l) \frac{\phi(x', \mu, \sigma)}{Z(a, b, \mu, \sigma)} dx' = C l \sqrt{2 \pi}\int_a^b \frac{\phi(x', \tilde{\mu}, \tilde{\sigma})}{Z(a, b, \mu, \sigma)} dx' = l \sqrt{2 \pi} C \frac{Z(a, b, \tilde{\mu}, \tilde{\sigma})}{Z(a, b, \mu, \sigma)},
\end{talign*}
where 
\begin{talign*}
	\tilde{\mu} = \frac{\mu l^2 + x \sigma^2}{\sigma^2 + l^2}, \qquad 
	\tilde{\sigma} = \sqrt{\frac{\sigma^2 l^2}{\sigma^2 + l^2}}, \qquad
	C = \frac{1}{\sqrt{2 \pi (\sigma^2 + l^2)}}\exp\left(\frac{(\mu - x)^2}{2 (\sigma^2 + l^2)}\right).
\end{talign*}

\subsection{Kernel Mean Embedding for Matern 1/2 Kernel}
\label{sec:matern}
For Gaussian distributions and the Matern 1/2 kernel, we can compute the posterior mean but only in $d=1$.
We provide the expression for the kernel mean embedding: $\Pi[k(\cdot, x)] = \int_{\mathbb{R}} k(x', x) \pi(x')dx'$, where $\pi(x) = \mathcal{N}(0, 1)$ is a standard normal and $k(x', x) = \exp(|x - x'|/l)$ is the Matern 1/2 kernel.
\begin{talign*}
	\Pi[k(\cdot, x)]=\frac{1}{2} \exp \left(\frac{2 x l + 1}{2l^2}\right) \mathrm{erfc} \left(\frac{x + \frac{1}{l}}{\sqrt{2}}\right) + \frac{1}{2} \exp \left(\frac{1 - 2xl}{2l^2}\right) \left(\mathrm{erf}\left(\frac{x - \frac{1}{l}}{\sqrt{2}}\right) + 1 \right)
\end{talign*}
