# Supplementary material for: Uncertainty and Structure in Neural Ordinary Differential Equations
Source: arXiv:2305.13290 source file (2023-05-22)
Supplement: Supplementary file 5 [file supp_exp_details.tex]

\section{EXPERIMENTAL DETAILS}

Below we give implementation details for all the datasets used and provide additional experimental results.

For our implementation of the BSN and the experiments described in the main text we make use of the following packages: \texttt{PyTorch} \citep{pytorch}, \texttt{emukit} \citep{paleyes2019emukit}, \texttt{GPyTorch} \citep{gpytorch}, \texttt{laplace-torch} \citep{daxberger2021laplace}, \texttt{PyWake}\citep{pywake}, and \texttt{Matplotlib} \citep{matplotlib}.

\subsection{Impact of Architecture Design}
\label{sec:sup_architecture}

We provide additional discussion concerning the choice of activation function, choice of sampling strategy and choice of optimizer.


\subsubsection{Choice of Optimizer}
\label{sec:optimizer}

We compare different optimizers for the BSN and a standard neural network, where for the standard neural network we use the same architecture as for $u_{\theta_u}$.
We use the 1-dimensional wind farm dataset with $n=320$ data points.
We choose this dataset, due to the complicated structure of the score function of a mixture of Gaussians.
For the experiment we consider three optimizers, i.e., Adam \citep{Kingma2015}, L-BFGS \citep{liu1989limited} and the Hessian-free optimizer \citep{martens2010deep}.
For Adam, we use mini-batching with a batch size of $32$ and full-batch training.
For the Hessian-free optimizer and L-BFGS we only consider full-batch training.
For Adam, we use $10000$ iterations, for the Hessian-free optimizer $1000$ iterations, and for L-BFGS we use automatic stopping based on the strong Wolfe conditions. 
We compare the loss for all training methods.
We also use CELU and RELU activation functions, where RELU is included as it is the standard activation function for neural networks.

Training a standard neural network with RELUs work significantly better, than using CELUs both in terms of the loss reached at the end of training and in terms of runtime (see Figure \ref{fig:regression_performance} and Figure \ref{fig:regression_performance_relu}).
Using RELUs does not work for the BSN, as the gradients of $u_{\theta_u}$ lead to discontinuities.

Training of the BSN using Adam is considerably slower than the training progress of the standard neural network.
We find that for CELU activation function, using (approximate) second order methods leads to a large improvement both in terms of speed and loss.
The success of the second order methods might be due to a narrow loss landscape, i.e., a larger spread in the eigenvalue spectrum of the curvature.
Therefore, we also examine the condition number of the Hessian, and we find that the BSN has a slightly higher condition number than the standard neural network (we do not report the condition number for RELUs as it cannot be computed numerically).
Given its short runtime and good optimization results, we choose L-BFGS for all our experiments.

\begin{figure}
\includegraphics{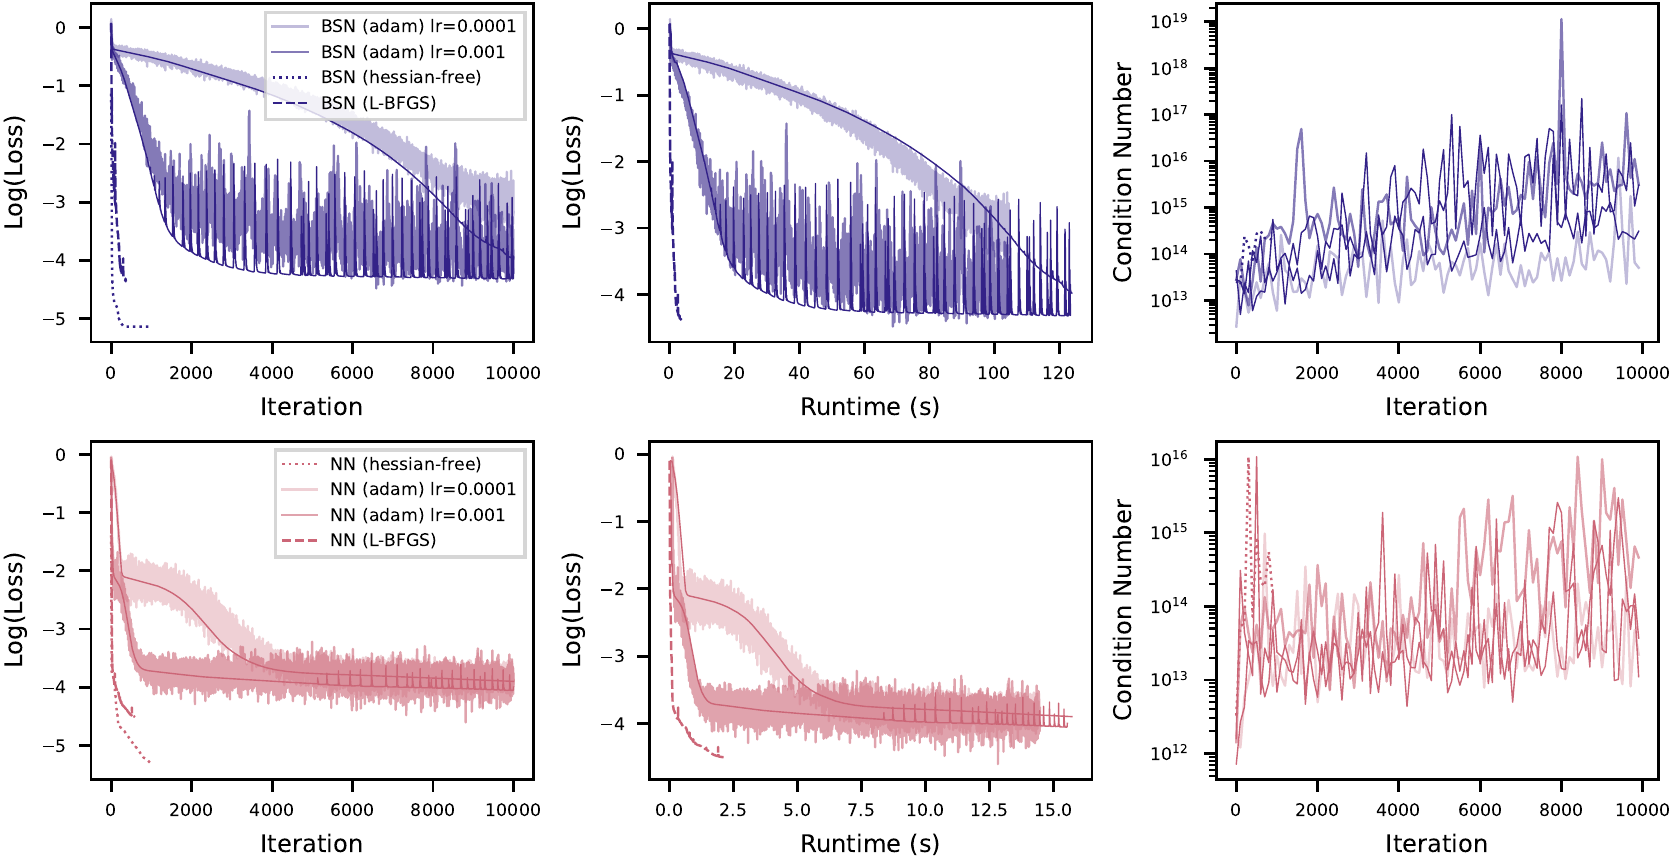}
\caption{Regression performance of a plain neural network (red) and a BSN (blue) using CELU activations. 
Loss (\emph{left}), and condition number (\emph{left}) as a function of the iteration. 
\emph{Centre:} loss as a function of the runtime.
Thin dark lines correspond to training with full-batch Adam.
Runtime of the Hessian-free optimizer not plotted, due to its long runtime.
}
\label{fig:regression_performance}
\end{figure}

\begin{figure}
\includegraphics{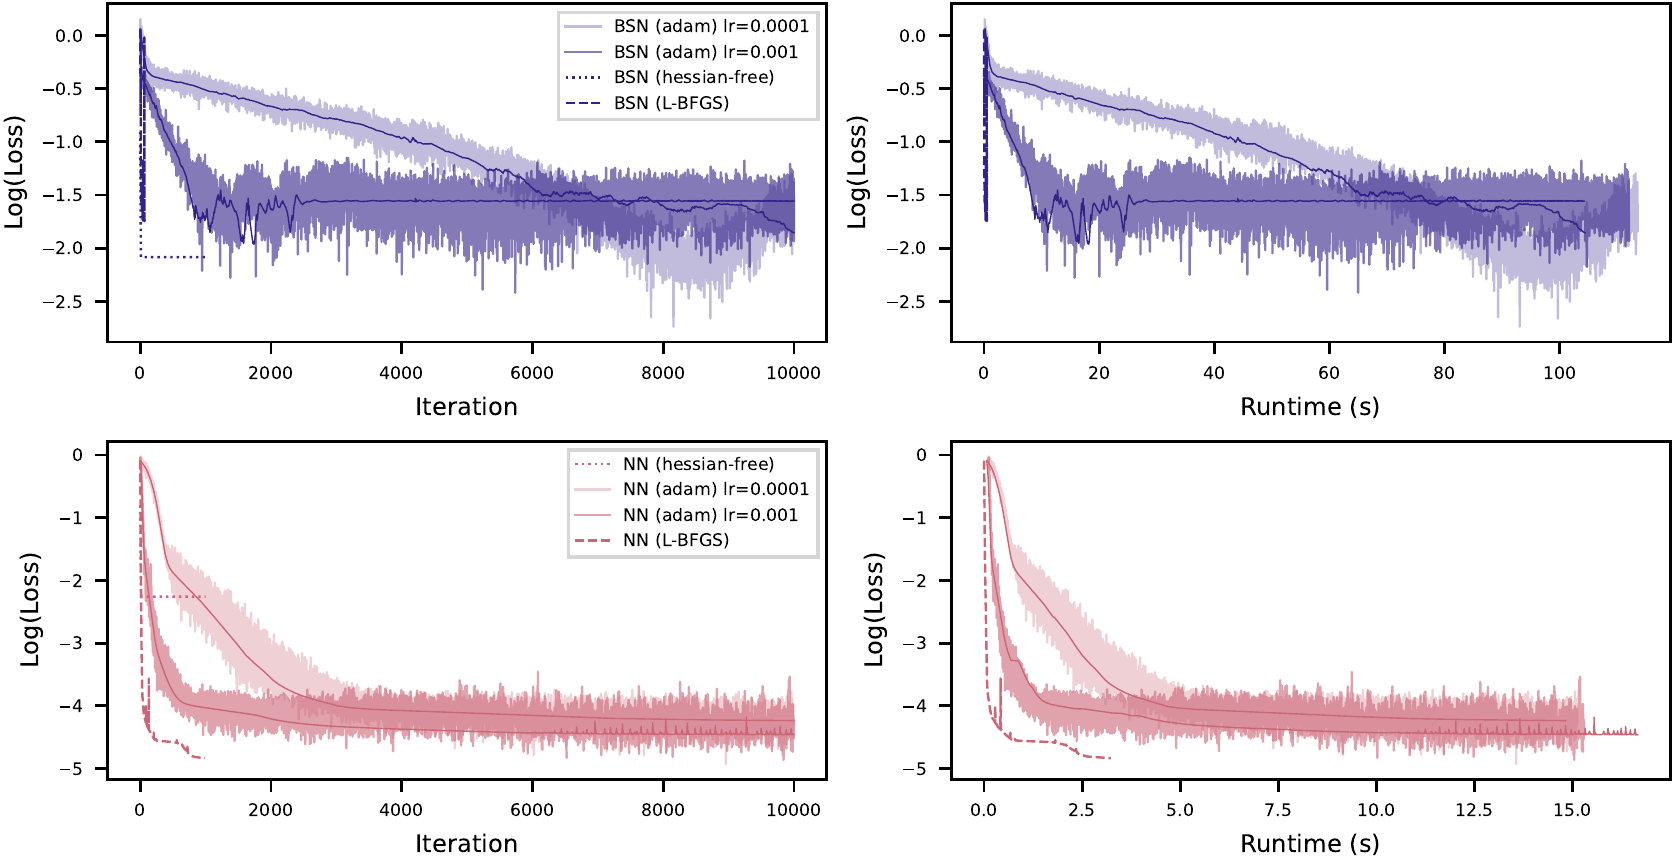}
\caption{Regression performance of a plain neural network (red) and a BSN (blue) using RELU activations. 
Loss (\emph{left}) as a function of the iteration. 
\emph{Centre:} loss as a function of the runtime.
Thin dark lines correspond to training with full-batch Adam.
Runtime of the Hessian-free optimizer not plotted, due to its long runtime.
}
\label{fig:regression_performance_relu}
\end{figure}

\subsubsection{Sampling Strategies}
\label{sec:sup_sampling}

For our experiments in the main text, we choose the data points by sampling from $\pi$, i.e., $x_i \sim \pi$.
Here we consider two additional sampling strategies:
\begin{itemize}
  \item Using a quasi-Monte Carlo (QMC) sequence. We use \texttt{SciPy}'s \citep{scipy} implementation of QMC based on the Sobol sequence \citep{sobol1967on}.
  \item Linearly spaced points in a hypercube (called \emph{grid} in Figure \ref{fig:genz_1_sampling}). Here we consider the hypercube $[-5 \sigma_{\pi}, 5 \sigma_{\pi}]^d$, where $\pi(x) = \mathcal{N}(x | 0, \sigma_{\pi})$.
\end{itemize}

Figure \ref{fig:genz_1_sampling} shows the result of the different sampling strategies in $d=1$.
The BSN performs better using MC samples then using QMC samples and grid points.
The low performance of the latter is expected, since too few points a placed in regions with a high probability mass.

\begin{figure}
\includegraphics{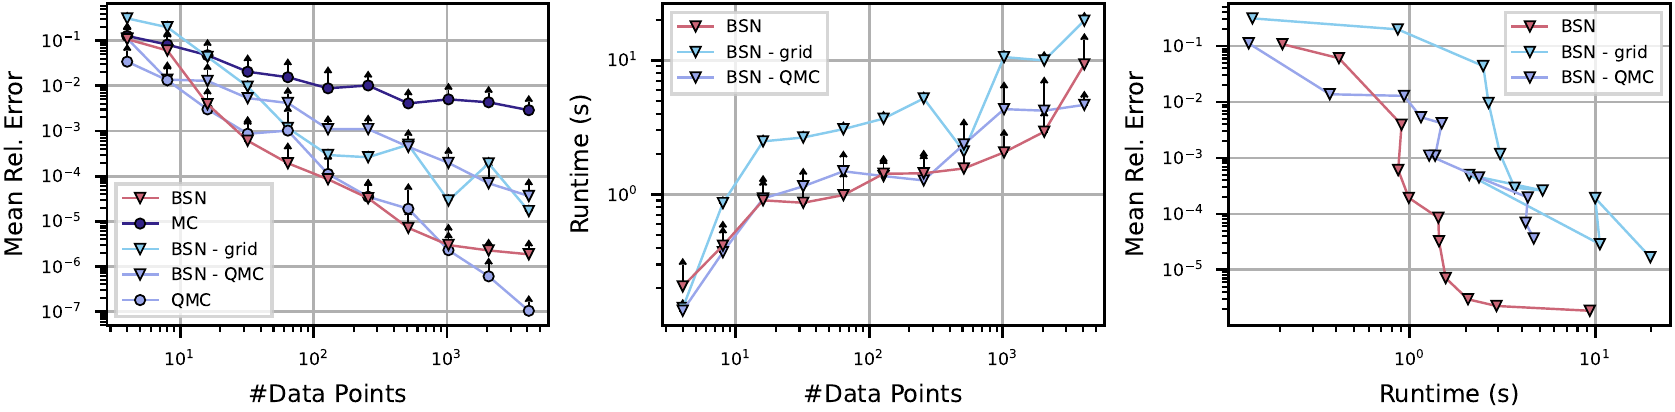}
\caption{Comparing different sampling schemes on the continuous Genz dataset in $d=1$. The BSN is trained on MC-sampled points, QMC-sampled points and on a regular grid.
  Mean relative integration error (\emph{left}), and runtime (\emph{centre}), (based on 5 repetitions) as a function of $n$. 
  \emph{Right:} Mean relative integration error as a function of runtime in seconds.
}
\label{fig:genz_1_sampling}
\end{figure}

\subsubsection{Choice of Architecture}
\label{sec:architecture_search}

We consider a basic architecture of the following form:
\begin{talign*}
    u_{\theta_u} = \text{Linear}(d, h) \circ CELU (\circ \text{Linear}(h, h) \circ CELU)^l \circ \text{Linear}(h, d), 
\end{talign*}
where $h$ are the number of hidden units and $l$ are the number of hidden layers.
Figure \ref{fig:architecture_search} shows the performance of different architectures on the 1-dimensional continuous Genz dataset.
All architectures perform similar but the architecture with $l=2$ and $h=32$ reaches the lowest error the fastest for large $n$.
Hence, we use this architecture for our experiments.

\begin{figure}
\includegraphics{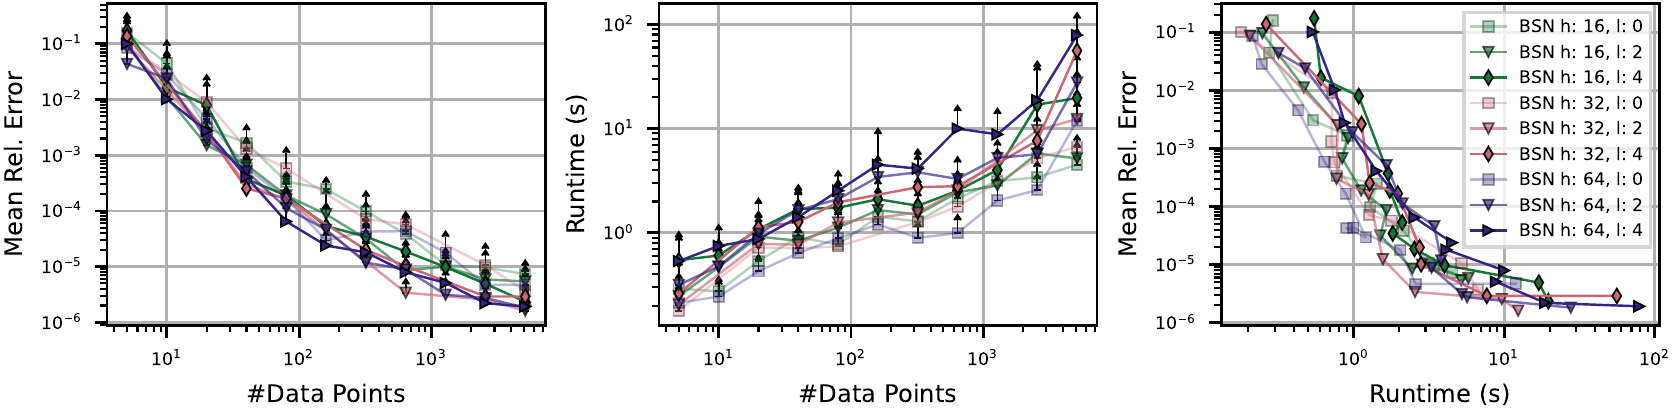}
\caption{
  Testing different architectures on the 1-dimensional continuous Genz dataset.
  Mean relative integration error (\emph{left}), and run time (\emph{centre}), (based on 5 repetitions) as a function of $n$. 
  \emph{Right:} Mean relative integration error as a function of run time in seconds.
}
\label{fig:architecture_search}
\end{figure}

\subsubsection{Choice of $m(x)$}
\label{sec:m_x}

For most of our experiments we set $m(x) = I_{d}$ in Equation~\eqref{eq:stein_operator}.
This might not necessarily be the best choice for a given task, but finding a function $m$ that works well is hard.
We test different $m$ on the 1-dimensional Continuous Genz function:
\begin{itemize}
  \item $m(x) = \frac{I_d}{||x||_2^2 +1}$ - $m(x)$ goes to zero for $x \rightarrow \pm\infty$
  \item $m(x) = \frac{I_d}{\sqrt{||x||_2^2 +1}}$ - $m(x)$ goes to zero for $x \rightarrow \pm\infty$ and cancels the $\nabla_x \log \pi(x)$ term for large $x$.
  \item $m(x) = I_d \pi(x)$ - in cases where $\pi$ is a normal distribution, this function also goes to zero for $x \rightarrow \pm\infty$.
  \item $m(x) = \mathrm{diag} x$ - example of a function having negative effect.
\end{itemize} 
The results of comparing these different $m$ are shown in Figure~\ref{fig:genz_m}.
On this test problem, none of the proposed $m$ significantly outperforms the choice $m(x)=I_d$, with some performing significantly worse.


\begin{figure}
\includegraphics{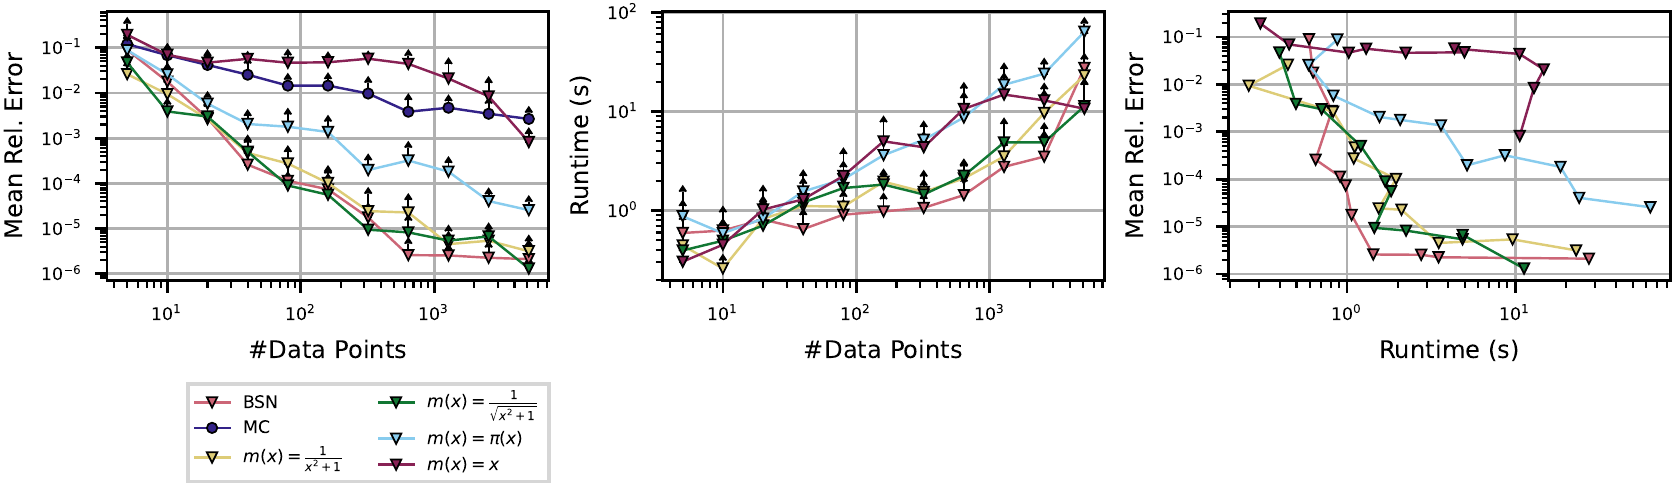}
\caption{\emph{Continuous Genz dataset in $d=1$ with different $m(x)$.}
Mean relative integration error (\emph{left}), run time (\emph{center}) (based on 5 repetitions) as a function of $n$. 
\emph{Right:} Mean relative integration error as a function of run time in seconds.
}
\label{fig:genz_m}
\end{figure}

\subsubsection{Choice of GP Kernel}
\label{sec:choice_kernel}
  As a benchmark we use BQ with an RBF kernel for all our experiments.
  The reason for this choice of kernel is the closed form availability of posterior mean and covariance when $\pi$ is a normal distribution.
  Here we add an experiment using a Matern 1/2 kernel.
  For this choice of kernel the posterior mean is only available in $d=1$, hence we conduct the experiment on the 1 dimensional Genz dataset (see Section~\ref{sec:matern} for the expression of the kernel mean embedding).
  The corresponding results a found in Figure~\ref{fig:genz_matern}. Once again, we do not observe a significant difference in performance, except for the continuous Genz dataset. 

\begin{figure}
\includegraphics{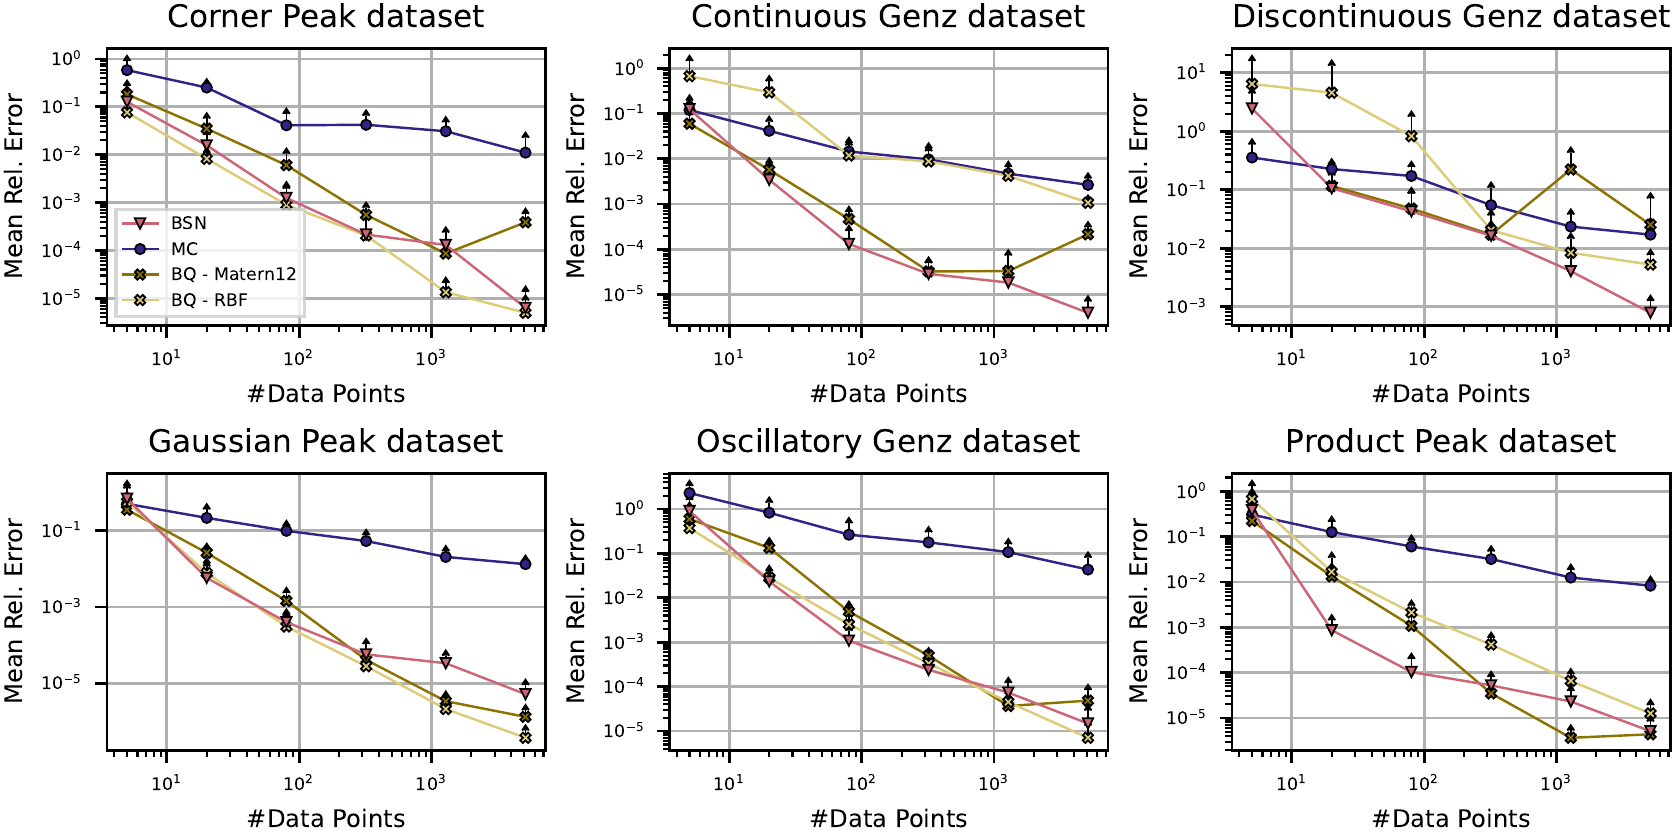}
\caption{\emph{BQ with Matern 1/2 kernel on the Genz family in $d=1$.}
Mean relative integration error (based on 5 repetitions) as a function of $n$. 
}
\label{fig:genz_matern}
\end{figure}

\subsection{Genz Benchmark}
\label{sec:genz_family}
\label{sec:exp_details_genz}
In our experiments we use the Genz integrand family dataset.
Here we include a short description of each dataset, plus additional experiments on the 2-dimensional version of each dataset.
In our experiments we integrate the Genz function against a standard normal $\pi(x) = \mathcal{N}(x | 0, 1)$.
This requires the transformation of the inputs to the original Genz functions $f$, which are to be integrated against $[0, 1]^d$.
Therefore, we compute $\Pi_{\pi}[f \circ c]$ where $c(x) = \frac{1}{2} \left( 1 + \text{erf} \left( \frac{x}{\sqrt{2}} \right) \right)$ is the cumulative density function of the standard normal.
We give the form of $f$ below.

\paragraph{Continuous Genz dataset}
The integrand is given by
\begin{talign*}
  f(x) = \exp \left( - \sum_{k=1}^d a_k | x_k - u_k| \right)
\end{talign*}
with parameters $a_k = 1.3$ and $u_k = 0.55$.
See Figure \ref{fig:genz_continuous} for results on a 2 dimensional version of this dataset.

\begin{figure}
\includegraphics{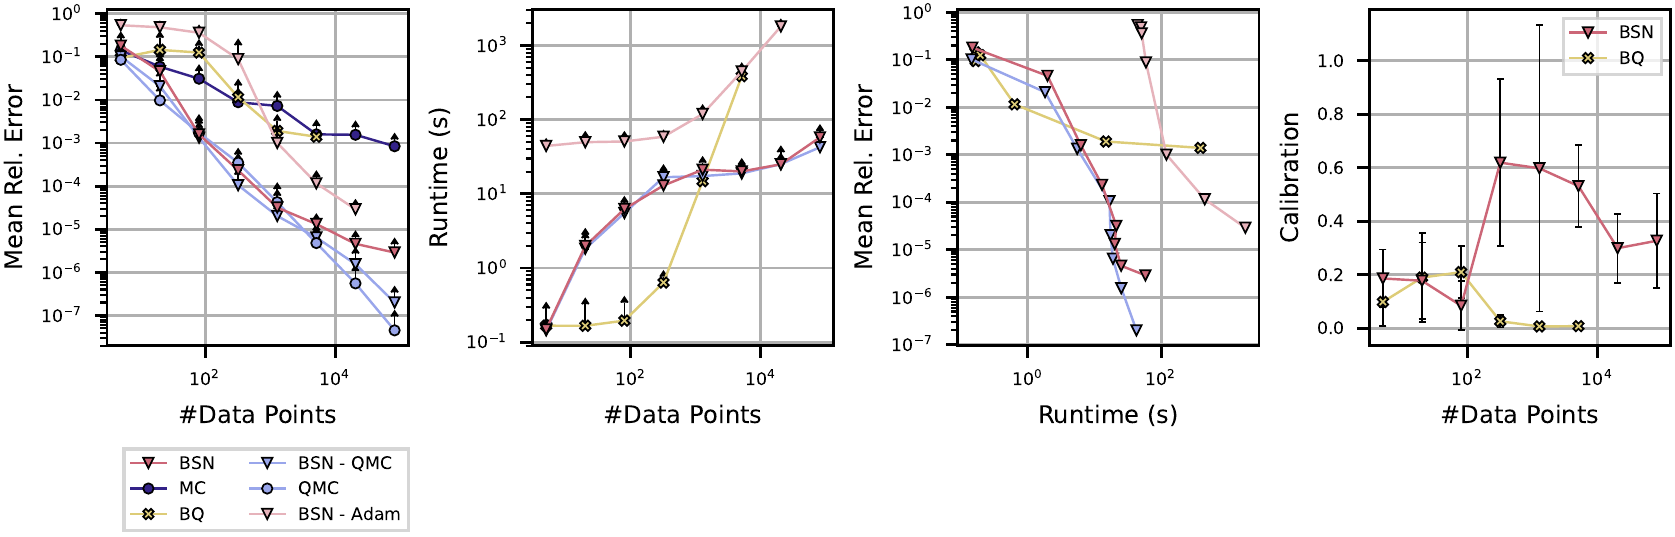}
\caption{\emph{Continuous Genz dataset in $d=2$.}
Mean relative integration error (\emph{left}), run time (\emph{centre-left}), and calibration (\emph{right}) (based on 5 repetitions) as a function of $n$. 
\emph{Center-right:} Mean relative integration error as a function of run time in seconds.
}
\label{fig:genz_continuous}
\end{figure}

\paragraph{Corner Peak dataset}
The integrand is given by
\begin{talign*}
  f(x) = \left(1 +  \sum_{k=1}^d a_k x_k \right)^{-(d+1)}
\end{talign*}
with parameters $a_k = 5$.
See Figure \ref{fig:genz_corner} for results on a 2 dimensional version of this dataset.

\begin{figure}
\includegraphics{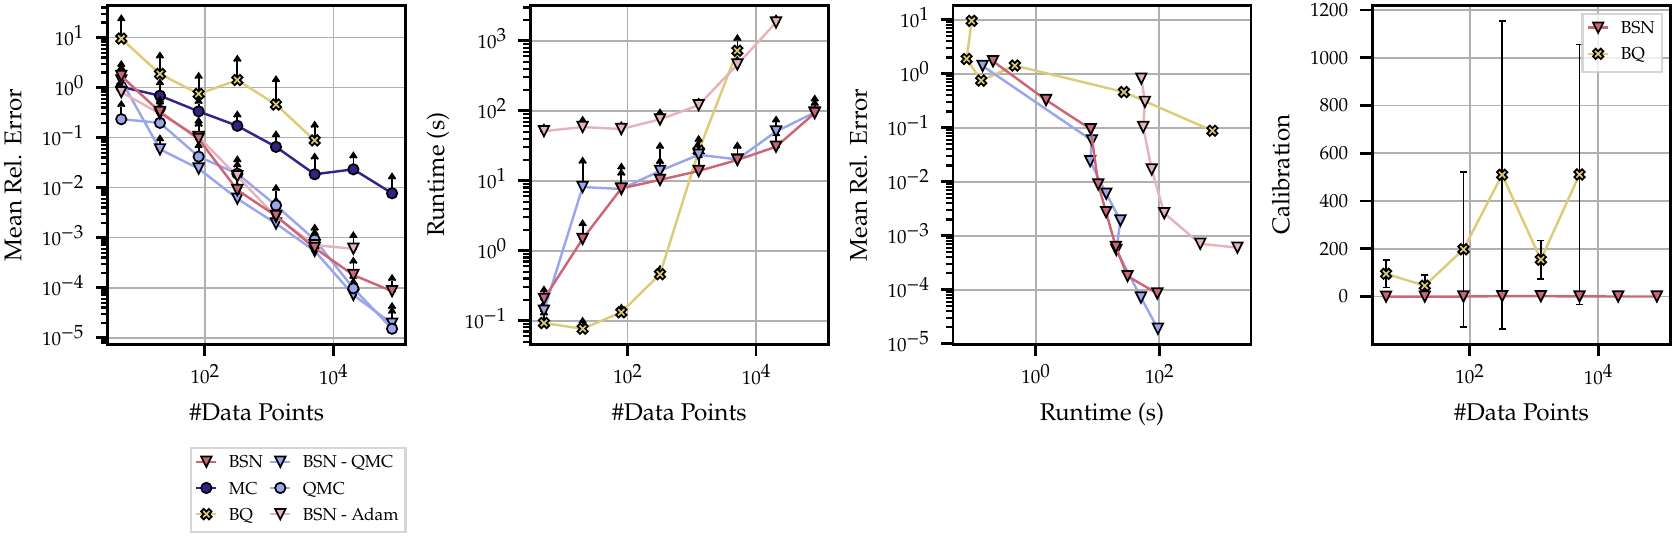}
\caption{\emph{Corner Peak dataset in $d=2$.}
Mean relative integration error (\emph{left}), run time (\emph{centre-left}), and calibration (\emph{right}) (based on 5 repetitions) as a function of $n$. 
\emph{Center-right:} Mean relative integration error as a function of run time in seconds.
}
\label{fig:genz_corner}
\end{figure}

\paragraph{Discontinuous Genz dataset}
The integrand is given by
\begin{talign*}
  f(x) = \begin{cases}
    0, \quad\text{if}~ x_k > u_k ~\text{for any}~ $k$\\
    \exp\left( \sum_{k=1}^d a_k x_k \right)
  \end{cases}
\end{talign*}
with parameters $a_k = 5$ and $u_k=0.5$.
See Figure \ref{fig:genz_discontinuous} for results on a 2 dimensional version of this dataset.

\begin{figure}
\includegraphics{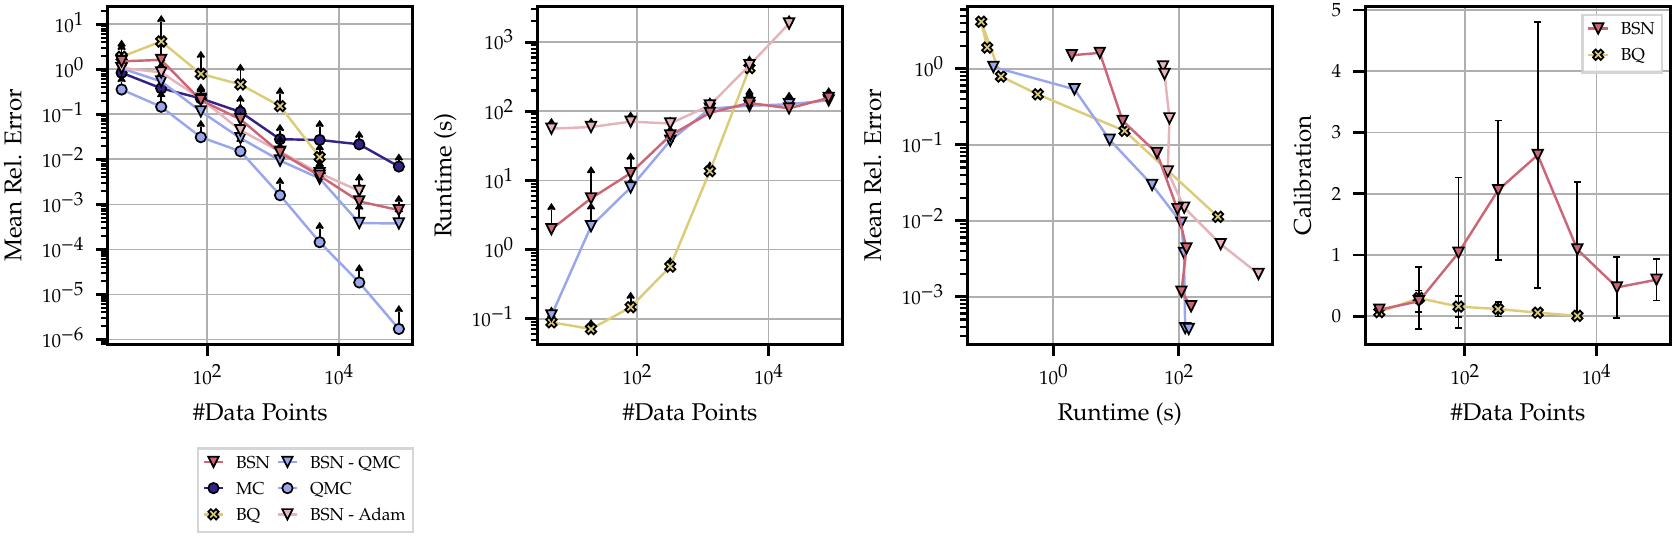}
\caption{\emph{Discontinuous Genz dataset in $d=2$.}
Mean relative integration error (\emph{left}), run time (\emph{centre-left}), and calibration (\emph{right}) (based on 5 repetitions) as a function of $n$. 
\emph{Center-right:} Mean relative integration error as a function of run time in seconds.
}
\label{fig:genz_discontinuous}
\end{figure}

\paragraph{Gaussian peak dataset}
The integrand is given by
\begin{talign*}
  f(x) = \exp \left( - \sum_{k=1}^d a_k^2 (x_k - u_k)^2 \right)
\end{talign*}
with parameters $a_k = 5$ and $u_k = 0.5$
See Figure \ref{fig:genz_gaussian} for results on a 2 dimensional version of this dataset.

\begin{figure}
\includegraphics{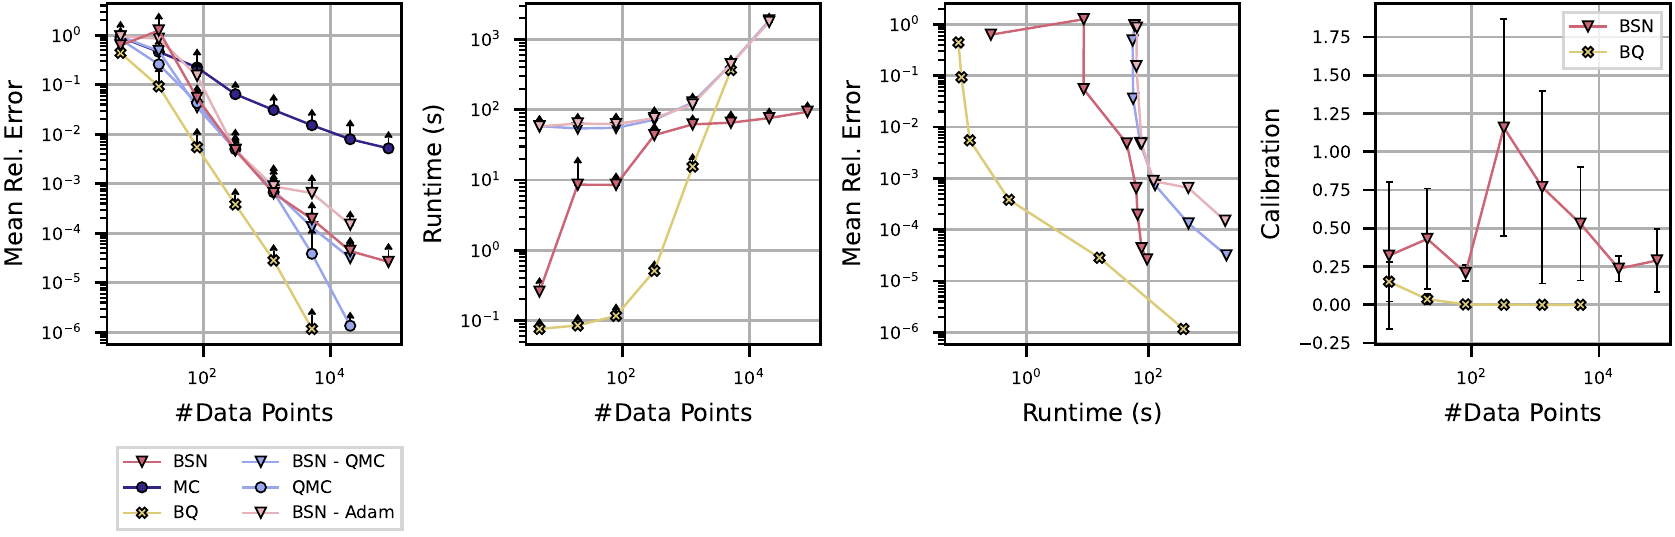}
\caption{\emph{Gaussian peak dataset in $d=2$.}
Mean relative integration error (\emph{left}), run time (\emph{centre-left}), and calibration (\emph{right}) (based on 5 repetitions) as a function of $n$. 
\emph{Center-right:} Mean relative integration error as a function of run time in seconds.
}
\label{fig:genz_gaussian}
\end{figure}

\paragraph{Product peak dataset}
The integrand is given by
\begin{talign*}
  f(x) = \prod_{k=1}^d \frac{1}{\left( a_k^{-2} + (x_k - u_k)^2\right)}
\end{talign*}
with parameters $a_k = 5$ and $u_k = 0.5$
See Figure \ref{fig:genz_product} for results on a 2 dimensional version of this dataset.

\begin{figure}
\includegraphics{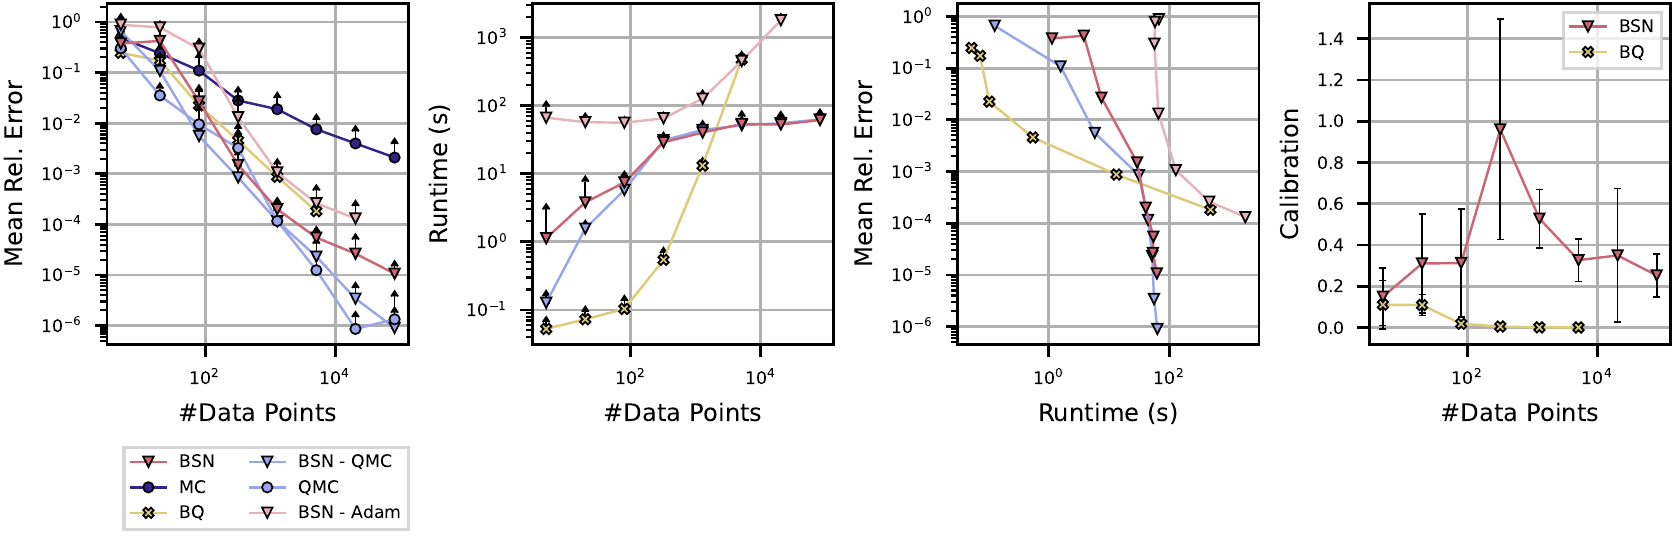}
\caption{\emph{Product peak dataset in $d=2$.}
Mean relative integration error (\emph{left}), run time (\emph{centre-left}), and calibration (\emph{right}) (based on 5 repetitions) as a function of $n$. 
\emph{Center-right:} Mean relative integration error as a function of run time in seconds.
}
\label{fig:genz_product}
\end{figure}

\paragraph{Oscillatory Genz dataset}
The integrand is given by
\begin{talign*}
  f(x) = \cos \left(2 \pi u + \sum_{k+1}^d a_k x_k \right)
\end{talign*}
with parameters $a_k = 5$ and $u = 0.5$
See Figure \ref{fig:genz_oscillatory} for results on a 2 dimensional version of this dataset.
\begin{figure}
\includegraphics{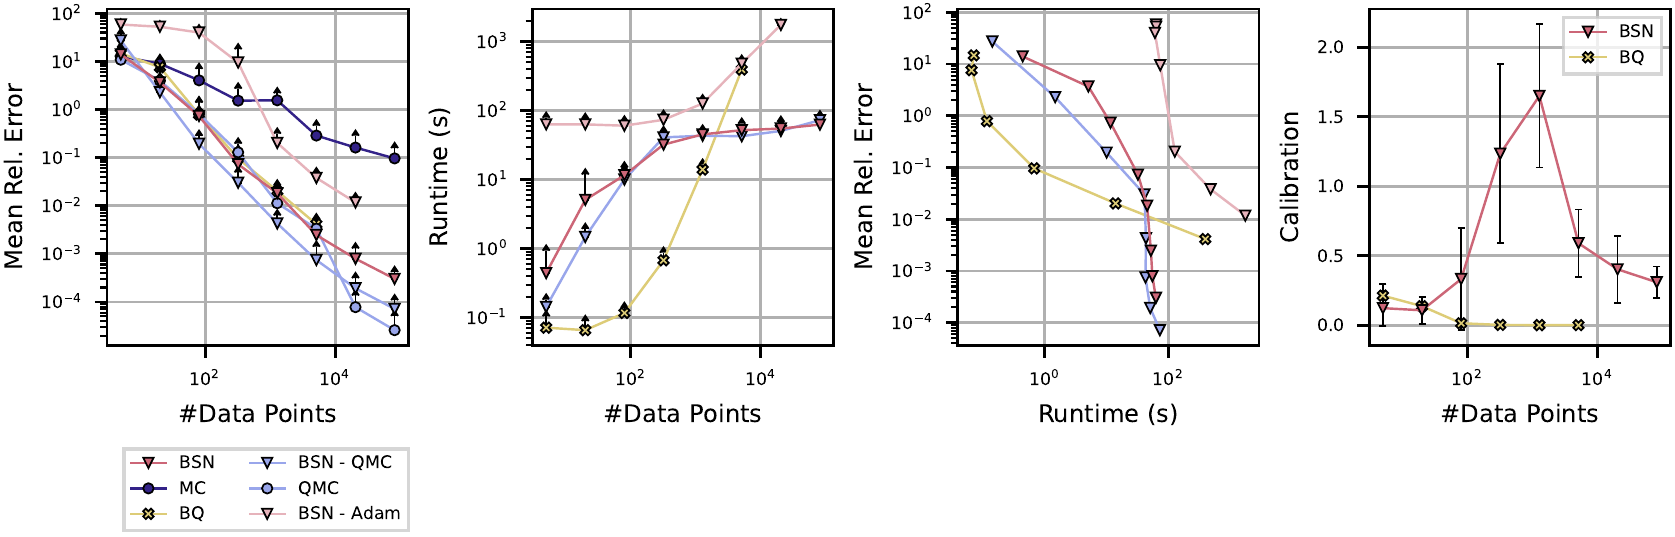}
\caption{
\emph{Oscillatory Genz dataset in $d=2$.}
Mean relative integration error (\emph{left}), run time (\emph{centre-left}), and calibration (\emph{right}) (based on 5 repetitions) as a function of $n$. 
\emph{Center-right:} Mean relative integration error as a function of run time in seconds.
  }
\label{fig:genz_oscillatory}
\end{figure}

\subsubsection{Memory Requirements}
\label{sec:genz_memory}
We can compare the BSN and BQ not only in runtime but also in terms of memory requirements.
However, computing accurate memory requirements in python can be difficult as common python libraries use for example \texttt{C++} backends.
The memory requirements of these non-python backends is commonly not taken into account using the built-in memory profiler.
So instead, we use the profiler of our cluster, which outputs the maximum memory required by the program.
Figure \ref{fig:memory} shows that the BSN memory requirements increase more slowly than for BQ.

\begin{figure}
\includegraphics{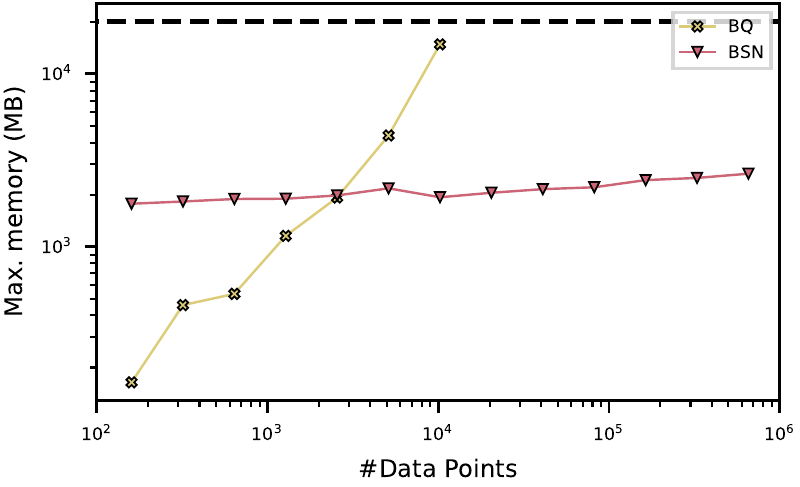}
\caption{Memory requirements of BQ and BSN on the continuous Genz dataset in $d=20$ (based on 5 repetitions).}
\label{fig:memory}
\end{figure}

\subsection{Goodwin Oscillator}
\label{sec:goodwin_oscillator}

Goodwin oscillator \citep{goodwin1965oscillatory} describes how the feedback loop between mRNA transcription and protein expression can lead to oscillatory dynamics in a cell. 
We here consider the case with no intermediate protein species.
The experimental setup is based on earlier work by \citep{Riabiz2020, chen2019stein, Calderhead2009, Oates2016thermo}.

The Goodwin oscillator with no intermediate protein species is given by:
\begin{talign*}
  \frac{du_1}{dt} &= \frac{a_1}{1 + a_2 u_2^\rho} - \alpha u_1\\
  \frac{du_2}{dt} &= k_1 u_1 - \alpha u_2,
\end{talign*}
where $u_1$ corresponds to the concentration of mRNA and $u_2$ to the concentration of the corresponding protein product.
We set $\rho = 10$.

As initial conditions we set $u_0 = (0, 0)$.
To generate the ground truth dataset, we set $a_1 = 1$, $a_2 = 3$, $k_1=1$ and $\alpha=0.5$.
We use a measurement noise of $\sigma = (0.1, 0.05)$.
Data was collected for $2400$ time points in $t\in[1, 25]$, leading to the following expression for the likelihood:
\begin{talign*}
 p(y | x) \propto \exp \left(- \frac{1}{2 \sigma_1^2} \sum_{k=1}^{2400} ||y_{1,k} - u_1(t_k) ||_2^2- \frac{1}{2 \sigma_2^2} \sum_{k=1}^{2400} ||y_{2,k} - u_2(t_k) ||_2^2 \right)
\end{talign*}
We use an \texttt{JAX}'s implementation of Dopri5(4) to solve the ODE. 
We use automatic differentiation implemented in \texttt{JAX} to compute derivatives of the likelihood with respect to the parameters.
To avoid parameters becoming negative, we use log-transformed parameters $w = \log(x)$ for the parameter inference via MCMC.
We place a standard normal prior on the log-transformed parameters $w$.
For each dataset we run five chains, where the initial conditions for each chain are sampled from the prior.

Figure \ref{fig:goodwin_oscillator2} shows the results for the remaining two parameters not shown in the main text.
\begin{figure*}
	\includegraphics{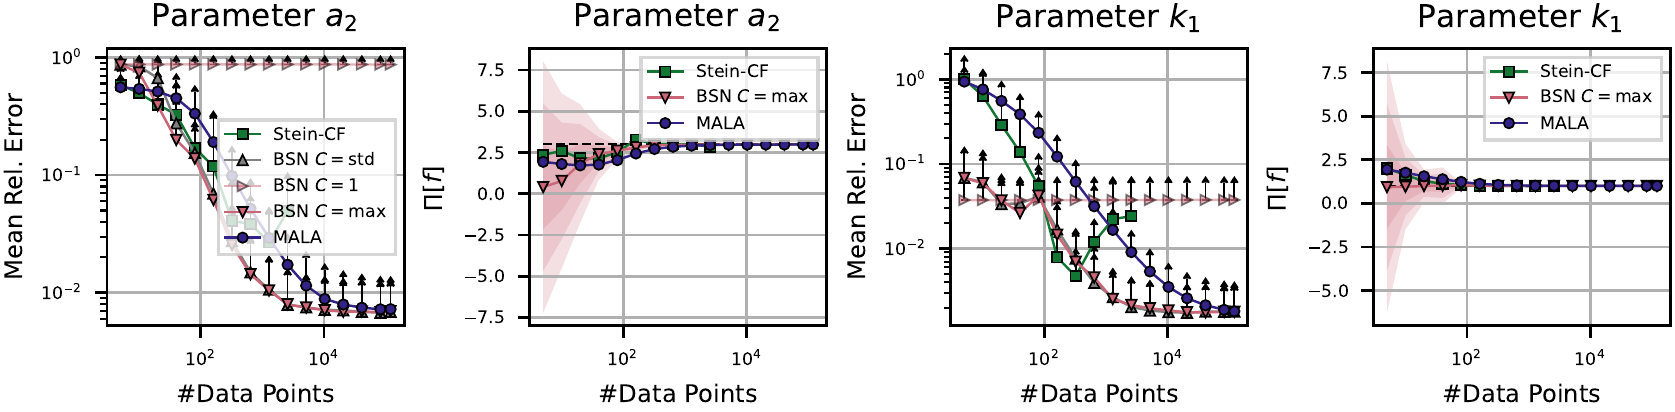}
	\caption{
  \emph{Posterior expectations for the parameters of a Goodwin ODE}.
  Mean relative integration error (\emph{left} and \emph{centre-right}), and uncertainty estimates (\emph{centre-left} and \emph{right}) (based on 5 repetitions) as a function of $n$. 
  }
	\label{fig:goodwin_oscillator2}
\end{figure*}

\subsection{Wind Farm Modelling}
\label{sec:exp_details_wind_farm}
For the wind farm model in our experiments, we assume we have a large-scale wind farm with equally spaced turbines on a two-dimensional grid and an ambient turbulence intensity. 
For each turbine, we use a wake deficit model by \citet{Niayifar2016}.
We put the following distributions on parameters for the wind farm simulation
\begin{itemize}
  \item \textbf{Turbine resistance coefficient:} Gaussian distribution with mean $\mu=1.33$ and variance $\sigma^2=0.1$.
  \item \textbf{Coefficient describing the wake expansion:} Gaussian distribution left-truncated at $0$ with mean $\mu=0.38$ and variance $\sigma = 0.001$.
  \item \textbf{Second coefficient describing the wake expansion:} Gaussian distribution left-truncated at $0$ with mean $\mu=4e-3$ and variance $\sigma^2=1e-8$.
  \item \textbf{Turbulence intensity:} Gaussian distribution left-truncated at $0$ with mean $\mu=0.1$ and variance $\sigma^2 = 0.003$
  \item \textbf{Wind direction:} Mixture of Gaussian distributions truncated so as to have support on $[0, 45]$ with means $\mu_1=0, \mu_2=22.5, \mu_3=33.75$ and variances $\sigma_1^2=50, \sigma_2^2=40, \sigma_3^2=8$.
  \item \textbf{Hub heights:} Gaussian distribution left-truncated at $0$ with mean $\mu=100$ and variance $\sigma^2=0.5$.
  \item \textbf{Hub diameter:} Gaussian distribution left-truncated at $0$ with mean $\mu=100$ and variance $\sigma^2=0.1$.
\end{itemize}

These distributions were chosen to have scales which might realistically represent uncertainty for their input, but if applying our method in practice these would have to be elicited from wind-farm experts. Note that the BSNs could be applied to much more complex distributions so-long as the density of $\Pi$ can be evaluated pointwise up to some normalization constant.

Our code is based on the code estimating the local turbine thrust coefficient \citet{Kirby2022} using a low-order wake model provided here: \url{https://github.com/AndrewKirby2/ctstar_statistical_model}. This code is based on the \texttt{PyWake} package \citep{pywake}.
