# Supplementary material for: Uncertainty and Structure in Neural Ordinary Differential Equations
Source: arXiv:2305.13290 source file (2023-05-22)
Supplement: Supplementary file 6 [file supp_laplace.tex]

\section{ADDITIONAL BACKGROUND: LAPLACE APPROXIMATION}
\label{sec:ggn_approx}
The Laplace approximation constructs a second-order Taylor approximation around the maximum of the posterior, i.e., the mode of the posterior, which amounts to a Gaussian approximate of the posterior around the MAP (maximum a-posteriori) estimate.
Here we provide a detailed introduction. 

We want to compute a posterior for the parameters of our model
\begin{talign}
  \begin{split}
  p(\theta| \mathcal{D}) &= \frac{p(\mathcal{D}| \theta)p(\theta)}{Z},\quad \text{where}\\
  Z &= \int p(\mathcal{D}| \theta)p(\theta) d\theta.
  \end{split}
  \label{eq:posterior}
\end{talign}
Here, the integral for the normalization constant $Z$ is usually not tractable, and we will have to resort to some approximation to compute it.
We provide the expressions for negative log prior
\begin{talign}
  - \log p(\theta) = \frac{1}{2 \sigma_0^2} \|\theta\|_2^2 - \frac{p+1}{2}\log \pi \sigma_0^2
  \label{eq:prior}
\end{talign}
and the negative log likelihood
\begin{talign}
  - \log p(\mathcal{D}|\theta) = \frac{1}{2 \sigma^2} \sum_{i=1}^n \|f(x_i) - g_\theta(x_i)\|_2^2 - \frac{n}{2}\log \pi \sigma^2,
  \label{eq:likelihood}
\end{talign}
where $\sigma$ is the dataset noise.
By comparing \eqref{eq:likelihood} and \eqref{eq:prior} to the mean square loss with weight decay
\begin{talign*}
    \begin{split}
        l_\text{tot}(\theta) & = l(\theta) + \lambda \|\theta\|_2^2 \\
        l(\theta) & = \frac{1}{n} \sum_{i=1}^n \|f(x_i) - g_\theta(x_i)\|_2^2
    \end{split}
\end{talign*}
we note $l \propto - \log p(\mathcal{D}| \theta)$ and $\lambda \|\theta\|_2^2 \propto - \log p(\theta)$.
Hence, the minimum of the loss correspond the maximum of the posterior, i.e. $\theta_{\text{MAP}} = \text{argmin}_{\theta} l_{\text{tot}}(\theta) = \text{argmin}_{\theta} -\log p(\mathcal{D}| \theta) - \log p(\theta) = \text{argmin}_{\theta} -\log p(\theta| \mathcal{D})$.  
We denote $L(\theta)  = \log p(\mathcal{D}| \theta) + \log p(\theta)$, and rewrite Equation \eqref{eq:posterior} 
\begin{talign*}
  p(\theta| \mathcal{D}) = \frac{e^{L(\theta)}}{Z}.  
\end{talign*}
To find a suitable approximation for the posterior we, we use as Taylor series expansion of $L$ around $\theta_{\text{MAP}}$
\begin{talign*}
  L(\theta) \approx L(\theta_\text{MAP}) + (\theta - \theta_\text{MAP})^\top \nabla_{\theta}L(\theta_{\text{MAP}})  + \frac{1}{2}(\theta - \theta_\text{MAP})^\top \nabla_{\theta}^2 L(\theta_{\text{MAP}}) (\theta - \theta_\text{MAP})
\end{talign*}
The second term is equal to zero by definition of $\theta_\text{MAP}$.
Hence, we arrive at a Gaussian approximation of the posterior $q(\theta)$ for the form
\begin{talign*}
 q_{\text{Laplace}}(\theta) = \mathcal{N}\left(\theta \mid \theta_\text{MAP}, \Sigma \right),
\end{talign*}
where $\Sigma$ is proportional to the inverse Hessian of the loss $l_{\text{tot}}$ evaluated at $\theta_\text{MAP}$: 
\begin{talign*}
 \Sigma^{-1} &=\nabla_{\theta}^2 L|_{\theta=\theta_{\text{MAP}}} 
 =  \left(- \nabla_\theta^2 \log p(\mathcal{D}|\theta) - \nabla_\theta^2 \log p(\theta)\right)|_{\theta=\theta_{\text{MAP}}}\\
 &= H  +  \sigma_0^{-2} I_{p+1}.
\end{talign*}
Since computing $H$ is computationally expensive, we use the GGN Approximation to compute it.

\subsection{GGN Approximation}
For the Laplace approximation we are interested in computing the Hessian of the log likelihood $-\log p(\mathcal{D}| \theta) \propto \frac{1}{2 \sigma^2} \sum_{i=1}^n \|f(x_i) - g_\theta(x_i)\|_2^2$.
The GGN approximation is a positive-semi-definite approximation of the full Hessian $H$, i.e.,
\begin{talign*}
  H &=  \nabla_{\theta}^2 \left(-\log p(\mathcal{D}| \theta)\right)\\
    &=  \nabla_{\theta}^2 \frac{1}{2 \sigma^2} \sum_{i=1}^n \|f(x_i) - g_\theta(x_i)\|_2^2 \\
    &= \frac{1}{2 \sigma^2} \sum_{i=1}^n \left[ \left(\nabla_{\theta} g_{\theta}(x_i)|_{\theta=\theta_{\text{MAP}}}\right)^\top 
    2 
    \nabla_{\theta} g_{\theta}(x_i)|_{\theta=\theta_{\text{MAP}}}
  + \nabla_{\theta}^2 g_{\theta}(x_i)|_{\theta=\theta_{\text{MAP}}} 
  \left(\nabla_g \|f(x_i) - g\|_2^2|_{g=g_{\theta_{\text{MAP}}}(x_i)}\right)^2 \right]\\
  &= H_{\text{GGN}} + R,
\end{talign*}
where $\sigma$ is the dataset noise as in Eq. \eqref{eq:likelihood}.
The GGN approximation is given by
\begin{talign*}
  H_{\text{GGN}} = \frac{1}{\sigma^2}\sum_{i=1}^n J(x_i)^\top J(x_i)
\end{talign*}
where $J(x_i) = \nabla_{\theta} g_{\theta}(x_i)|_{\theta=\theta_{\text{MAP}}}$.
